# Supplementary material for: Don't Miss the Forest for the Trees: Attentional Vision Calibration for Large Vision Language Models
Source: arXiv:2405.17820 source file (2025-05-31)
Supplement: Supplementary file 1 [file additional_analysis.tex]

\begin{figure*}[t!]
    \centering
    \vspace{-3mm}
    \includegraphics[width=\textwidth]{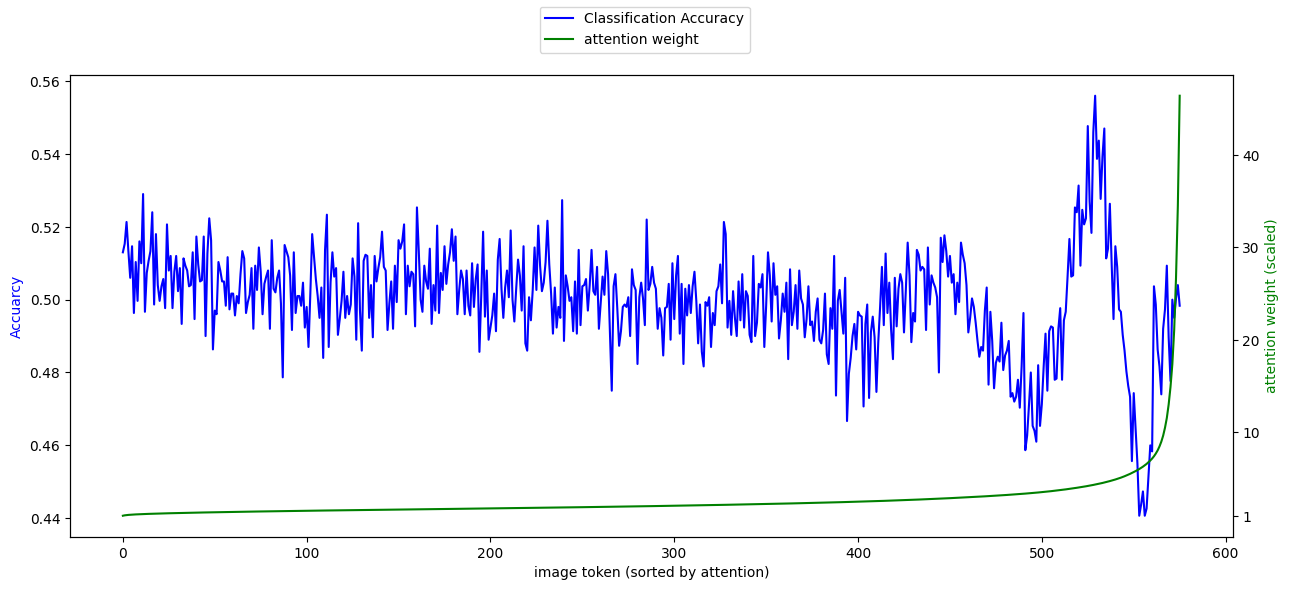}
    \vspace{\abovefigcapmargin}
    \caption{
    \textbf{Capability of image token in LVLMs.}
    \todo{POPE benchmark는 "Is there <object> in the image?"의 prompt를 통해 주어진 이미지 속 특정 object의 존재 판단 능력을 측정하는 benchmark이다.
이는 하나의 binary classification 문제로서 바라 볼 수 있고, 이에 대해 각 image token의 last value의 LLMs head를 통한 classification accuarcy를 attention에 대해 sort하여 나타내보았고(a), logit 평균이 정답에 더 기여한 횟수를 blind token vs non blind token에 비교하여 분석해보았다(b). }
    % 딱히 query (\textsc{Q})에 대한 정보가 없는 이미지 (\textsc{V})에도 특정 image token에 bias 되는 현상이 있음.
    % 첫 token을 generation할 때를 기준으로 모든 layer에 대해 attention weight를 average함.
    }%
    \label{fig:observation_bias}
    \vspace{\belowfigcapmargin}
\end{figure*}
